# Supplementary material for: Topological Phases in AB-Stacked MoTe$_2$/WSe$_2$: $\mathbb{Z}_2$ Topological Insulators, Chern Insulators, and Topological Charge Density Waves
Source: arXiv:2111.01152 source file (2022-08-09)
Supplement: Supplementary file 1 [file SM.pdf]

# Supplemental material for "Topological Phases in AB-stacked $MoTe_2/WSe_2$: $\mathbb{Z}_2$ Topological Insulators, Chern Insulators, and Topological Charge Density Waves"

Haining Pan,[1] Ming Xie,[1] Fengcheng Wu,[2,3,*] and Sankar Das Sarma[1]

[1] *Condensed Matter Theory Center and Joint Quantum Institute, Department of Physics, University of Maryland, College Park, Maryland 20742, USA*
[2] *School of Physics and Technology, Wuhan University, Wuhan 430072, China*
[3] *Wuhan Institute of Quantum Technology, Wuhan 430206, China*

## SINGLE-PARTICLE HAMILTONIAN

The single-particle Hamiltonian in the second quantization formalism can be expressed as

$$\hat{\mathcal{H}}_0 = \sum_{\tau=\pm} \int d^2\boldsymbol{r}\Psi_\tau^\dagger(\boldsymbol{r}) H_\tau \Psi_\tau(\boldsymbol{r}), \tag{S1}$$

$$H_\tau = \begin{pmatrix} -\frac{\hbar^2\boldsymbol{k}^2}{2m_\mathfrak{b}} + \Delta_{\mathfrak{b},\tau}(\boldsymbol{r}) & \Delta_{\mathrm{T},\tau}(\boldsymbol{r}) \\ \Delta_{\mathrm{T},\tau}^\dagger(\boldsymbol{r}) & -\frac{\hbar^2(\boldsymbol{k}-\tau\boldsymbol{\kappa})^2}{2m_\mathfrak{t}} + \Delta_{\mathfrak{t},\tau}(\boldsymbol{r}) + V_{z\mathfrak{t}} \end{pmatrix}, \tag{S2}$$

$$\Psi_+(\boldsymbol{r}) = \begin{pmatrix} \psi_{\mathfrak{b},\uparrow,+}(\boldsymbol{r}) \\ \psi_{\mathfrak{t},\downarrow,+}(\boldsymbol{r}) \end{pmatrix}, \quad \Psi_-(\boldsymbol{r}) = \begin{pmatrix} \psi_{\mathfrak{b},\downarrow,-}(\boldsymbol{r}) \\ \psi_{\mathfrak{t},\uparrow,-}(\boldsymbol{r}) \end{pmatrix}, \tag{S3}$$

where $\tau = \pm$ represents $\pm K$ valleys, $\hbar\boldsymbol{k} = -i\hbar\partial_{\boldsymbol{r}}$ is the momentum operator, $\boldsymbol{\kappa} = \frac{4\pi}{3a_M}(1,0)$ is at a corner of the moiré Brillouin zone (as shown in Fig. S1), and $a_M$ is the moiré lattice constant. Note that the spin index of the fermion operators $\Psi_\tau$ is both layer and valley dependent.

The Hamiltonian $\hat{\mathcal{H}}_0$ respects the time reversal symmetry $\mathcal{T}$, which is defined as

$$\hat{\mathcal{T}}\psi_{l,s,\tau}(\boldsymbol{r})\hat{\mathcal{T}}^{-1} = -\sum_{s'} \epsilon_{ss'}\psi_{l,s',-\tau}(\boldsymbol{r}), \quad \hat{\mathcal{T}}\psi_{l,s,\tau}^\dagger(\boldsymbol{r})\hat{\mathcal{T}}^{-1} = -\sum_{s'} \epsilon_{ss'}\psi_{l,s',-\tau}^\dagger(\boldsymbol{r}), \quad \hat{\mathcal{T}}i\hat{\mathcal{T}}^{-1} = -i, \tag{S4}$$

where $\hat{\mathcal{T}}$ is an antiunitary operator, the layer index $l = \{\mathfrak{b}, \mathfrak{t}\}$ for the bottom and top layer, the spin index $s = \{\uparrow, \downarrow\}$ for spin up and down, and $\epsilon_{ss'}$ is the totally antisymmetric tensor with $\epsilon_{\uparrow\downarrow} = -\epsilon_{\downarrow\uparrow} = 1$. Here the $\hat{\mathcal{T}}$ operation flips both spin and valley indices. By imposing the $\mathcal{T}$ symmetry $\hat{\mathcal{T}}\hat{\mathcal{H}}_0\hat{\mathcal{T}}^{-1} = \hat{\mathcal{H}}_0$, we find the following constraints

$$\Delta_{l,-\tau}(\boldsymbol{r}) = \Delta_{l,\tau}^*(\boldsymbol{r}), \quad \Delta_{\mathrm{T},-\tau}(\boldsymbol{r}) = -\Delta_{\mathrm{T},\tau}^*(\boldsymbol{r}), \tag{S5}$$

Because the Hamiltonian $H_\tau$ is Hermitian, $\Delta_{l,\tau}(\boldsymbol{r}) = \Delta_{l,\tau}^*(\boldsymbol{r})$. Therefore, $\Delta_{l,-}(\boldsymbol{r}) = \Delta_{l,+}(\boldsymbol{r})$, and we can denote the intralayer potential simply as $\Delta_l(\boldsymbol{r})$ by dropping the valley index. For the interlayer tunneling at $+K$ valley $\Delta_{\mathrm{T},+}(\boldsymbol{r}) = w\left(1 + \omega e^{i\boldsymbol{g}_2\cdot\boldsymbol{r}} + \omega^2 e^{i\boldsymbol{g}_3\cdot\boldsymbol{r}}\right)$, we obtain the tunneling at $-K$ valley as $\Delta_{\mathrm{T},-}(\boldsymbol{r}) = -w\left(1 + \omega^{-1}e^{-i\boldsymbol{g}_2\cdot\boldsymbol{r}} + \omega^{-2}e^{-i\boldsymbol{g}_3\cdot\boldsymbol{r}}\right)$, where $\omega = e^{i\frac{2\pi}{3}}$, and we assume $w$ takes a real value. The form of $\Delta_{T,+}(\boldsymbol{r})$ is determined by $C_{3z}$ (threefold rotation) symmetry.

Parameters of the single-particle Hamiltonian $H_\tau$ have been obtained through density-functional-theory(DFT) band structure calculation [1]. However, the obtained parameters $(w, V_b)$ are of the order of meV, which are likely too small to be accurately estimated by DFT. Therefore, we treat $(w, V_b)$ as adjustable parameters. The main physical picture that we obtain in this work remains valid if we vary $(w, V_b)$, which we have checked numerically. In addition, these parameters could be tunable by pressure applied between layers.

## HARTREE-FOCK CALCULATION

In this section, we include the Coulomb interaction and derive the mean-field Hamiltonian by applying the Hartree-Fock (HF) approximation. We first rewrite $\hat{\mathcal{H}}_0$ in the momentum space with the creation operator being defined as $c_{\boldsymbol{k},l,\tau}^\dagger = \frac{1}{\sqrt{A}}\int \psi_{l,\tau}^\dagger(\boldsymbol{r})e^{i\boldsymbol{k}\cdot\boldsymbol{r}}d^2\boldsymbol{r}$ (the spin index is absent because it can be inferred from the valley and layer indices due to the effective spin-valley-layer locking), where $A$ is the total area. Thus, $\hat{\mathcal{H}}_0$ can be expressed as

$$\hat{\mathcal{H}}_0 = \sum_{\boldsymbol{k}_\alpha,\boldsymbol{k}_\beta}\sum_{l_\alpha,l_\beta}\sum_\tau h_{\boldsymbol{k}_\alpha l_\alpha,\boldsymbol{k}_\beta l_\beta}^{(\tau)} c_{\boldsymbol{k}_\alpha,l_\alpha,\tau}^\dagger c_{\boldsymbol{k}_\beta,l_\beta,\tau}, \tag{S6}$$

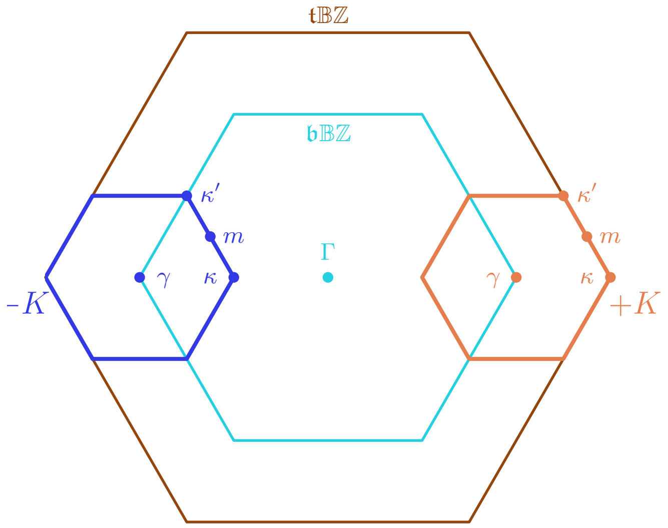


FIG. S1. A schematic illustration of the momentum space structure. The cyan and brown hexagons represent the Brillouin zone of $MoTe_2$ (bottom layer) and $WSe_2$ (top layer), respectively. The small hexagon on the right (left) is the moiré Brillouin zone for $+K$ ($-K$) valley. Note that we use a different convention of the moiré Brillouin zone from that in Ref. [1] due to a gauge transformation which puts the center of the moiré Brillouin zone ($\gamma$ point) at the corner of the bottom layer Brillouin zone. We exaggerate the difference between $MoTe_2$ and $WSe_2$ Brillouin zones for illustration.

where $h^{(\tau)}$ is the Hamiltonian $H_\tau$ expanded in the plane-wave basis, and the momentum $\boldsymbol{k}$ is defined in the extended Brillouin zone that spans the full momentum space, i.e., $\boldsymbol{k} \in \mathbb{R}^2$. Here, the subscripts $\alpha, \beta$ are index for momenta. Due to Bloch's theorem, $h^{(\tau)}_{\boldsymbol{k}_\alpha l_\alpha, \boldsymbol{k}_\beta l_\beta}$ is nonzero only when $\boldsymbol{k}_\alpha - \boldsymbol{k}_\beta$ is equal to the linear combination of any multiples of hone of the moiré reciprocal lattice vectors (including the zero vector).

At the charge neutrality (filling factor $\nu = 0$) of the heterobilayer, all valence bands are below Fermi energy. We are interested in situations where the valence bands are slightly hole-doped. Therefore, it is convenient to study the many-body interaction in the hole basis. We define the hole operator as $b_{\boldsymbol{k},l,\tau} = c^\dagger_{\boldsymbol{k},l,\tau}$, and $\hat{\mathcal{H}}_0$ in the hole basis is

$$\hat{\mathcal{H}}_0 = \sum_\tau \operatorname{Tr} h^{(\tau)} - \sum_{\boldsymbol{k}_\alpha, \boldsymbol{k}_\beta} \sum_{l_\alpha, l_\beta} \sum_\tau [h^{(\tau)}]^\intercal_{\boldsymbol{k}_\alpha l_\alpha, \boldsymbol{k}_\beta l_\beta} b^\dagger_{\boldsymbol{k}_\alpha, l_\alpha, \tau} b_{\boldsymbol{k}_\beta, l_\beta, \tau} \tag{S7}$$

By combing the single-particle Hamiltonian with the hole-hole Coulomb interaction term, we obtain the full Hamiltonian (dropping the constant term) as

$$\begin{aligned} \hat{\mathcal{H}} &= \hat{\mathcal{H}}_1 + \hat{\mathcal{H}}_{\text{int}}, \\ \hat{\mathcal{H}}_1 &= \sum_{\boldsymbol{k}_\alpha, \boldsymbol{k}_\beta} \sum_{l_\alpha, l_\beta} \sum_\tau \tilde{h}^{(\tau)}_{\boldsymbol{k}_\alpha l_\alpha, \boldsymbol{k}_\beta l_\beta} b^\dagger_{\boldsymbol{k}_\alpha, l_\alpha, \tau} b_{\boldsymbol{k}_\beta, l_\beta, \tau}, \\ \hat{\mathcal{H}}_{\text{int}} &= \frac{1}{2A} \sum_{\boldsymbol{k}_\alpha, \boldsymbol{k}_\beta, \boldsymbol{k}_\gamma, \boldsymbol{k}_\delta} \sum_{l_\alpha, l_\beta} \sum_{\tau_\alpha, \tau_\beta} V(\boldsymbol{k}_\alpha - \boldsymbol{k}_\delta) b^\dagger_{\boldsymbol{k}_\alpha, l_\alpha, \tau_\alpha} b^\dagger_{\boldsymbol{k}_\beta, l_\beta, \tau_\beta} b_{\boldsymbol{k}_\gamma, l_\beta, \tau_\beta} b_{\boldsymbol{k}_\delta, l_\alpha, \tau_\alpha} \delta_{\boldsymbol{k}_\alpha + \boldsymbol{k}_\beta, \boldsymbol{k}_\delta + \boldsymbol{k}_\gamma}, \end{aligned} \tag{S8}$$

where $\tilde{h}^{(\tau)} = -[h^{(\tau)}]^\intercal$, the dual-gate screened Coulomb interaction $V(\boldsymbol{k}) = 2\pi e^2 \tanh(|\boldsymbol{k}|d)/(\epsilon|\boldsymbol{k}|)$, $d$ is the sample-to-gate distance, and $\epsilon$ is the dielectric constant.

Using the HF approximation, we obtain the following mean-field Hamiltonian $\hat{H}^{\text{HF}}$,

$$\begin{aligned} \hat{\mathcal{H}}^{\text{HF}} &= \hat{\mathcal{H}}_1 + \hat{\mathcal{H}}^{\text{HF}}_{\text{int}}, \\ \hat{\mathcal{H}}^{\text{HF}}_{\text{int}} &= \frac{1}{A} \sum_{\boldsymbol{k}_\alpha, \boldsymbol{k}_\beta, \boldsymbol{k}_\gamma, \boldsymbol{k}_\delta} \sum_{l_\alpha, l_\beta} \sum_{\tau_\alpha, \tau_\beta} V(\boldsymbol{k}_\alpha - \boldsymbol{k}_\delta) \Big( \Big\langle b^\dagger_{\boldsymbol{k}_\alpha, l_\alpha, \tau_\alpha} b_{\boldsymbol{k}_\delta, l_\alpha, \tau_\alpha} \Big\rangle b^\dagger_{\boldsymbol{k}_\beta, l_\beta, \tau_\beta} b_{\boldsymbol{k}_\gamma, l_\beta, \tau_\beta} \\ &\quad - \Big\langle b^\dagger_{\boldsymbol{k}_\alpha, l_\alpha, \tau_\alpha} b_{\boldsymbol{k}_\gamma, l_\beta, \tau_\beta} \Big\rangle b^\dagger_{\boldsymbol{k}_\beta, l_\beta, \tau_\beta} b_{\boldsymbol{k}_\delta, l_\alpha, \tau_\alpha} \Big) \delta_{\boldsymbol{k}_\alpha + \boldsymbol{k}_\beta, \boldsymbol{k}_\delta + \boldsymbol{k}_\gamma}. \end{aligned} \tag{S9}$$

The Hartree-Fock solution can either preserve or spontaneously break the moiré lattice translational symmetry. In our study, we always assume that the interaction-induced states have a real-space unit cell that is commensurate with

the moiré unit cell, but the former can be larger than the latter, for example in charge/spin density wave states. In $\hat{\mathcal{H}}_{\rm int}^{\rm HF}$, the average value $\left\langle b^{\dagger}_{\boldsymbol{k}_\alpha,l_\alpha,\tau_\alpha} b_{\boldsymbol{k}_\beta,l_\beta,\tau_\beta}\right\rangle$ is nonzero only when $\boldsymbol{k}_\alpha - \boldsymbol{k}_\beta = \boldsymbol{G}$, where $\boldsymbol{G}$ is a reciprocal lattice vector (including the zero vector) of the resulting real-space unit cell.

The total energy per moiré unit cell is obtained by averaging $\hat{H}$ in Eq. (S8), i.e.,

$$\begin{aligned}
\left\langle \hat{\mathcal{H}} \right\rangle &= \left\langle \hat{\mathcal{H}}_1 \right\rangle + \left\langle \hat{\mathcal{H}}_{\rm int} \right\rangle, \\
\left\langle \hat{\mathcal{H}}_1 \right\rangle &= \sum_{\boldsymbol{k}_\alpha,\boldsymbol{k}_\beta} \sum_{l_\alpha,l_\beta} \sum_{\tau} \tilde{h}^{(\tau)}_{\boldsymbol{k}_\alpha l_\alpha,\boldsymbol{k}_\beta l_\beta} \left\langle b^{\dagger}_{\boldsymbol{k}_\alpha,l_\alpha,\tau} b_{\boldsymbol{k}_\beta,l_\beta,\tau} \right\rangle, \\
\left\langle \hat{\mathcal{H}}_{\rm int} \right\rangle &= \frac{1}{2A} \sum_{\boldsymbol{k}_\alpha,\boldsymbol{k}_\beta,\boldsymbol{k}_\gamma,\boldsymbol{k}_\delta} \sum_{l_\alpha,l_\beta} \sum_{\tau_\alpha,\tau_\beta} V(\boldsymbol{k}_\alpha - \boldsymbol{k}_\delta) \Big( \left\langle b^{\dagger}_{\boldsymbol{k}_\alpha,l_\alpha,\tau_\alpha} b_{\boldsymbol{k}_\delta,l_\alpha,\tau_\alpha} \right\rangle \left\langle b^{\dagger}_{\boldsymbol{k}_\beta,l_\beta,\tau_\beta} b_{\boldsymbol{k}_\gamma,l_\beta,\tau_\beta} \right\rangle \\
&\quad - \left\langle b^{\dagger}_{\boldsymbol{k}_\alpha,l_\alpha,\tau_\alpha} b_{\boldsymbol{k}_\gamma,l_\beta,\tau_\beta} \right\rangle \left\langle b^{\dagger}_{\boldsymbol{k}_\beta,l_\beta,\tau_\beta} b_{\boldsymbol{k}_\delta,l_\alpha,\tau_\alpha} \right\rangle \Big) \delta_{\boldsymbol{k}_\alpha+\boldsymbol{k}_\beta,\boldsymbol{k}_\delta+\boldsymbol{k}_\gamma},
\end{aligned} \tag{S10}$$

## NUMERICAL CALCULATION OF CHERN NUMBER

In this section, we briefly introduce the numerical technique to calculate the Chern number [2, 3]. For a non-degenerate band characterized by the wavefunction $|u_n(\boldsymbol{k})\rangle$, the Chern number of the $n$-th band is defined as

$$\mathcal{C}_n = \frac{1}{2\pi} \int_{1\mathbb{BZ}} \Omega_n(\boldsymbol{k}) \mathrm{d}^2 k, \tag{S11}$$

where the Berry curvature $\Omega_n(\boldsymbol{k}) = \partial_x A_{n,y}(\boldsymbol{k}) - \partial_y A_{n,x}(\boldsymbol{k})$, and the Berry connection $A_{n,\mu}(\boldsymbol{k}) = -i \langle u_n(\boldsymbol{k})|\partial_\mu|u_n(\boldsymbol{k})\rangle$.

The direct way of calculation Eq. (S11) by differentiating the wavefunction $|u_n(\boldsymbol{k})\rangle$ is numerically unstable because the gauge-dependent berry connection $\boldsymbol{A}_n(\boldsymbol{k})$ is not guaranteed to be continuous. Therefore, we resort to a gauge-independent method by first discretizing the first Brillouin zone $1\mathbb{BZ}$ into small nonoverlapping plaquettes $\Gamma_i$ (i.e., $\cup_i \Gamma_i = 1\mathbb{BZ}$, $\Gamma_i \cap \Gamma_j = \Gamma_i \delta_{i,j}$) as per

$$\mathcal{C}_n = \frac{1}{2\pi} \sum_i \int_{\Gamma_i} \Omega_n(\boldsymbol{k}) \mathrm{d}^2 k = \frac{1}{2\pi} \sum_i \oint_{\partial \Gamma_i} \mathrm{d}\boldsymbol{k} \cdot \boldsymbol{A}_n(\boldsymbol{k}). \tag{S12}$$

For a sufficiently small plaquette enclosed by the loop $\partial\Gamma_i = (\boldsymbol{k}_{i,1}, \boldsymbol{k}_{i,2}, \ldots, \boldsymbol{k}_{i,s}, \boldsymbol{k}_{i,s+1} = \boldsymbol{k}_{i,1})$, the flux of Berry curvature $\Phi_{n,i} = \int_{\Gamma_i} \Omega_n(\boldsymbol{k}) \mathrm{d}^2 k$ can be approximated by finite differences followed by computing its exponential,

$$\begin{aligned}
e^{i\Phi_{n,i}} &= e^{\oint_{\partial\Gamma_i} \mathrm{d}\boldsymbol{k}^\mu \langle u_n(\boldsymbol{k})|\partial_\mu|u_n(\boldsymbol{k})\rangle} = \prod_s e^{\delta k^\mu_{i,s} \langle u_n(\boldsymbol{k}_{i,s})|\partial_\mu|u_n(\boldsymbol{k}_{i,s})\rangle} \approx \prod_s \left(1 + \delta k^\mu_{i,s} \langle u_n(\boldsymbol{k}_{i,s})|\partial_\mu|u_n(\boldsymbol{k}_{i,s})\rangle\right) \\
&\approx \prod_s \langle u_n(\boldsymbol{k}_{i,s})|u_n(\boldsymbol{k}_{i,s+1})\rangle,
\end{aligned} \tag{S13}$$

which is manifestly gauge invariant. Thus, the flux on $\Gamma_i$ is simply the angle of Eq. (S13), i.e.,

$$\Phi_{n,i} = \arg \prod_s \langle u_n(\boldsymbol{k}_{i,s})|u_n(\boldsymbol{k}_{i,s+1})\rangle, \tag{S14}$$

and the Chern number is obtained by summing up all fluxes on small plaquettes $\Gamma_i$,

$$\mathcal{C}_n = \frac{1}{2\pi} \sum_i \Phi_{n,i}. \tag{S15}$$

In our calculation, we solve the wavefunction $|u_n(\boldsymbol{k})\rangle$ self-consistently from the Hamiltonian (S9), and discretize the first Brillouin zone using a Monkhorst-Pack grid of 15 by 15. [4]

## MEAN-FIELD ANSATZ

We perform the Hartree-Fock calculation using an iterative approach. We start from an ansatz, i.e., an initial guess state (a Slater determinant state). The average value $\left\langle b^{\dagger}_{\boldsymbol{k}_\alpha,l_\alpha,\tau_\alpha} b_{\boldsymbol{k}_\beta,l_\beta,\tau_\beta}\right\rangle$ is calculated with respect to this ansatz, and we obtain the first generation of $\hat{\mathcal{H}}^{\mathrm{HF}}$, which is diagonalized to obtain the next generation of state. This process is iterated until the convergence of the total energy is reached. We discuss choices of the ansatz in different situations in the following.

For states at $\nu = 2$, we diagonalize $\tilde{h}^{(\tau)}$, and take an ansatz in which the lowest energy band of $\tilde{h}^{(\tau)}$ at each valley is occupied and other states are empty. This ansatz preserves the $\mathcal{T}$ symmetry.

For the valley polarized (VP) state at $\nu = 1$, we set a similar initial ansatz with the difference being that only the lowest band at $+K$ valley is fully occupied, which explicitly breaks the $\mathcal{T}$ symmetry. This initial ansatz will evolve to VP trivial insulator, VP Chern insulator or VP metallic state depending on the band offset $V_{z\mathfrak{t}}$.

For the intervalley coherent phases, e.g., the SDW and FM$_x$ at $\nu = 1$, we use an ancillary Hamiltonian $h_{\text{ansatz}}$ to generate the initial ansatz, and $h_{\text{ansatz}}$ has the following form

$$\begin{aligned} h_{\text{ansatz}} &= \begin{pmatrix} \tilde{h}^{(+)} & 0 \\ 0 & \tilde{h}^{(-)} \end{pmatrix} + \delta h_{\text{ansatz}} \\ \delta h_{\text{ansatz}} &= \alpha(\boldsymbol{S}\cdot\vec{\tau}) \otimes \left(\frac{1+\sigma_z}{2}\right), \end{aligned} \tag{S16}$$

where $\vec{\tau}$ is the vector of the Pauli matrices acting on the valley space, and $\sigma_z$ is the $z$-component Pauli matrix acting on the layer space, and $\alpha$ is an energy constant. For simplicity, we choose $\delta h_{\text{ansatz}}$ such that it only acts on the bottom layer.

For the in-plane FM$_x$ state, we choose $\boldsymbol{S} = (1, 0, 0)$ such that spin polarization in the bottom layer is along an in-plane direction, which leads to

$$\delta h^{(\mathrm{FM}_x)}_{\text{ansatz}} = \alpha\tau_x \otimes \left(\frac{1+\sigma_z}{2}\right) = \alpha \begin{pmatrix} 0&0&1&0\\0&0&0&0\\1&0&0&0\\0&0&0&0 \end{pmatrix}. \tag{S17}$$

For the SDW state, the moiré lattice translational symmetry is broken so that the system has a $\sqrt{3}\times\sqrt{3}$ period. We assume that the three MM sites in the new enlarged unit cell carry an in-plane antiferromagnetic Néel spin ordering, which can have two chiralities $\chi = \pm 1$ (denoted by SDW1 and SDW2 in Fig. 3 in the main text). We define the spin texture as $\boldsymbol{S} = \sum_{j=1}^{3} (\cos(\chi\boldsymbol{q}_j\cdot\boldsymbol{r}), \sin(\chi\boldsymbol{q}_j\cdot\boldsymbol{r}), 0)$, where $\boldsymbol{q}_j = \frac{4\pi}{\sqrt{3}a_M}\left(\cos\left(\frac{2\pi(j-1)}{3}\right), \sin\left(\frac{2\pi(j-1)}{3}\right)\right)$. This spin texture Hamiltonian is given by

$$\delta h^{(\mathrm{SDW})}_{\text{ansatz}}(\chi) = \alpha\sum_{j=1}^{3}\cos(\chi\boldsymbol{q}_j\cdot\boldsymbol{r})\tau_x\otimes\left(\frac{1+\sigma_z}{2}\right) + \sin(\chi\boldsymbol{q}_j\cdot\boldsymbol{r})\tau_y\otimes\left(\frac{1+\sigma_z}{2}\right) = \alpha\sum_{j=1}^{3}\begin{pmatrix} 0&0&e^{-i\chi\boldsymbol{q}_j\cdot\boldsymbol{r}}&0\\0&0&0&0\\e^{i\chi\boldsymbol{q}_j\cdot\boldsymbol{r}}&0&0&0\\0&0&0&0 \end{pmatrix}. \tag{S18}$$

In Fig. 3(a) in the main text, besides the SDW1 and SDW2, we find another SDW (denoted by SDW3) in the phase diagram which has the same chirality as SDW1 but has a charge density redistribution within one super unit cell. The SDW1 ansatz evolves to SDW3 for parameter regions where the SDW3 phase is favored.

For the two phases at $\nu = 2/3$ (FM$_z$ and AF$_z$), the charge order forms a honeycomb lattice with a period of $\sqrt{3}\times\sqrt{3}$, which can be generated by

$$\delta h^{(\nu=2/3)}_{\text{ansatz}} = \alpha\sum_{j=1}^{3}\begin{pmatrix} \cos(\boldsymbol{q}_j\cdot\boldsymbol{r}+\phi)+V & 0 & 0 & 0\\ 0&0&0&0\\ 0&0&\cos(\boldsymbol{q}_j\cdot\boldsymbol{r}-\phi)&0\\ 0&0&0&0 \end{pmatrix}. \tag{S19}$$

For FM$_z$, we choose $\alpha < 0$, $\phi = \pi$ and $V > 0$ such that valley-dependent potential in Eq. (S19) reaches its minimum at two vertices of a honeycomb lattice in real space and only at $+K$ valley in the valley pseudospin space. For AF$_z$, we choose $\alpha < 0$, $\phi = 2\pi/3$ and $V = 0$; then the valley-dependent potential in Eq. (S19) reaches its minimum in one vertex of the honeycomb lattice for $+K$ valley and the other vertex for $-K$ valley.

## ENERGIES OF COMPETING STATES

The phase diagrams in the main text are obtained by choosing the lowest energy state among all competing states. In this section, we explicitly show the energy per moiré unit cell of competing states at $\nu = 1$ and $\nu = 2/3$, where the energy is calculated according to Eq. (S10). Moreover, we present the corresponding charge density (CD) and spin density (SD) on both layers of every competing state in the real space.

For $\nu = 1$, we show the average energies per moiré unit cell of the competing states at $\epsilon = 12$ and $\epsilon = 17$ in Fig. S2(a) and S2(b), respectively. These competing states appear in the phase diagram of Fig. 3 in the main text.

In Fig. S2(a), at a small $|V_{zt}|$, the energetic favorable state is in-plane ferromagnetism ($FM_x$). For generic values of $V_{zt}$, there are actually two types of in-plane ferromagnetic states, $FM_x$ and $FM'_x$, as indicated by the light yellow line ($V_{zt} < -12$ meV) and the yellow line ($V_{zt} > -12$ meV) in Fig. S2(a), respectively. These two phases differ in the localization of holes. The holes tend to be localized at XX for a small negative $V_{zt}$ in $FM_x$ [Fig. S3], while they are localized at MM for a large negative $V_{zt}$ in $FM'_x$ [Fig. S4].

As $V_{zt}$ decreases towards more negative values, the energetically favorable state becomes the valley polarized state (VP), of which the CD and SD are shown in Fig. S5. Finally, the energetically favorable state becomes SDW1 at a large negative $V_{zt}$, of which the CD and SD are shown in Fig. S6.

For a larger dielectric constant, for example, at $\epsilon = 17$, the two kinds of spin density waves (i.e., SDW2 and SDW3) become energetically favorable. The CD and SD for SDW2 and SDW3 are shown in Figs. S7 and S8, respectively.

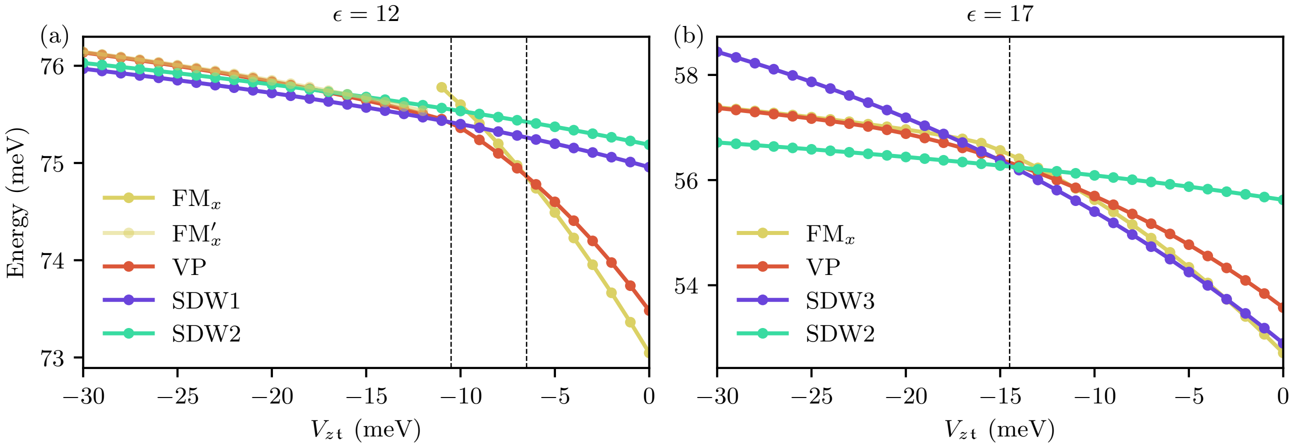


FIG. S2. $\nu = 1$. The energies per moiré unit cell as a function of $V_{zt}$ at (a) $\epsilon = 12$ and (b) $\epsilon = 17$. The competing states are: (i) $FM_x$ (yellow) or $FM'_x$ (light yellow); (ii) VP (red); (iii) SDW1 ($\epsilon = 12$, blue) or SDW3 ($\epsilon = 17$, blue); (iv) SDW2 (green).

Figure S9 shows the average energies per moiré unit cell of the competing states at $\nu = 2/3$. There are three competing states, (i)$AF_z$-HC, (ii) $FM_z$-HC, and (iii) $FM_z$, of which the CD and SD are shown in Figs. S10, S11, and S12, respectively. The $FM_z$-HC and $AF_z$-HC states have, respectively, antiferromagnetic and ferromagnetic spin ordering on a generalized Wigner crystal with honeycomb lattice on the bottom layer. The $FM_z$ state has ferromagnetic spin ordering and respects the moiré lattice translational symmetry.

* wufcheng@whu.edu.cn

[1] Y. Zhang, T. Devakul, and L. Fu, Spin-textured Chern bands in AB-stacked transition metal dichalcogenide bilayers, PNAS **118**, 10.1073/pnas.2112673118 (2021).
[2] F. Wu and S. Das Sarma, Quantum geometry and stability of moiré flatband ferromagnetism, Phys. Rev. B **102**, 165118 (2020).
[3] T. Fukui, Y. Hatsugai, and H. Suzuki, Chern Numbers in Discretized Brillouin Zone: Efficient Method of Computing (Spin) Hall Conductances, J. Phys. Soc. Jpn. **74**, 1674 (2005).
[4] H. J. Monkhorst and J. D. Pack, Special points for Brillouin-zone integrations, Phys. Rev. B **13**, 5188 (1976).

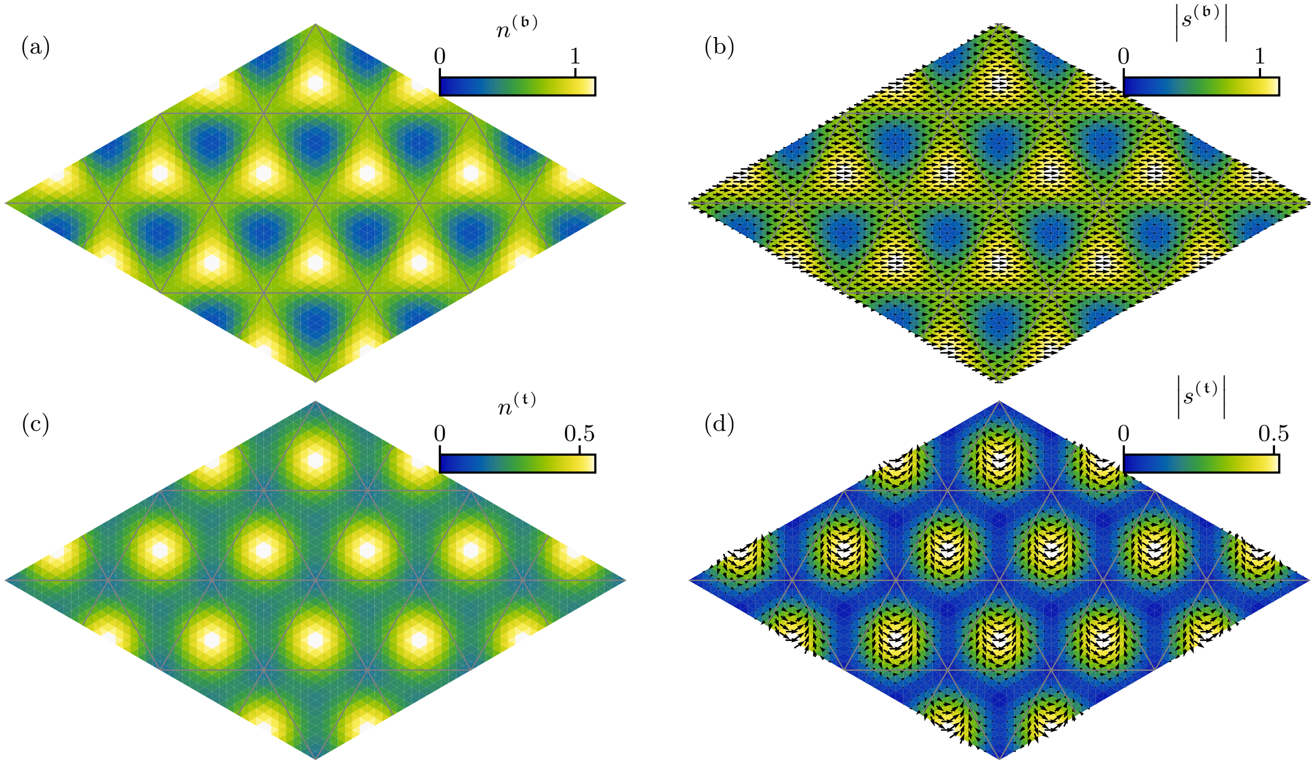


FIG. S3. $\nu = 1$. The charge density waves and spin density waves of $\mathrm{FM}_x$ at $V_{z\mathfrak{t}} = -1$ meV and $\epsilon = 12$. The first column shows the hole density $n$ on the bottom (a) and top layer (c); the second column shows the in-plane spin texture with the false color indicating the magnitude on the bottom (b) and top layer (d), respectively($s_z$ vanishes). The gray solid lines connect MM points in the moiré lattice.

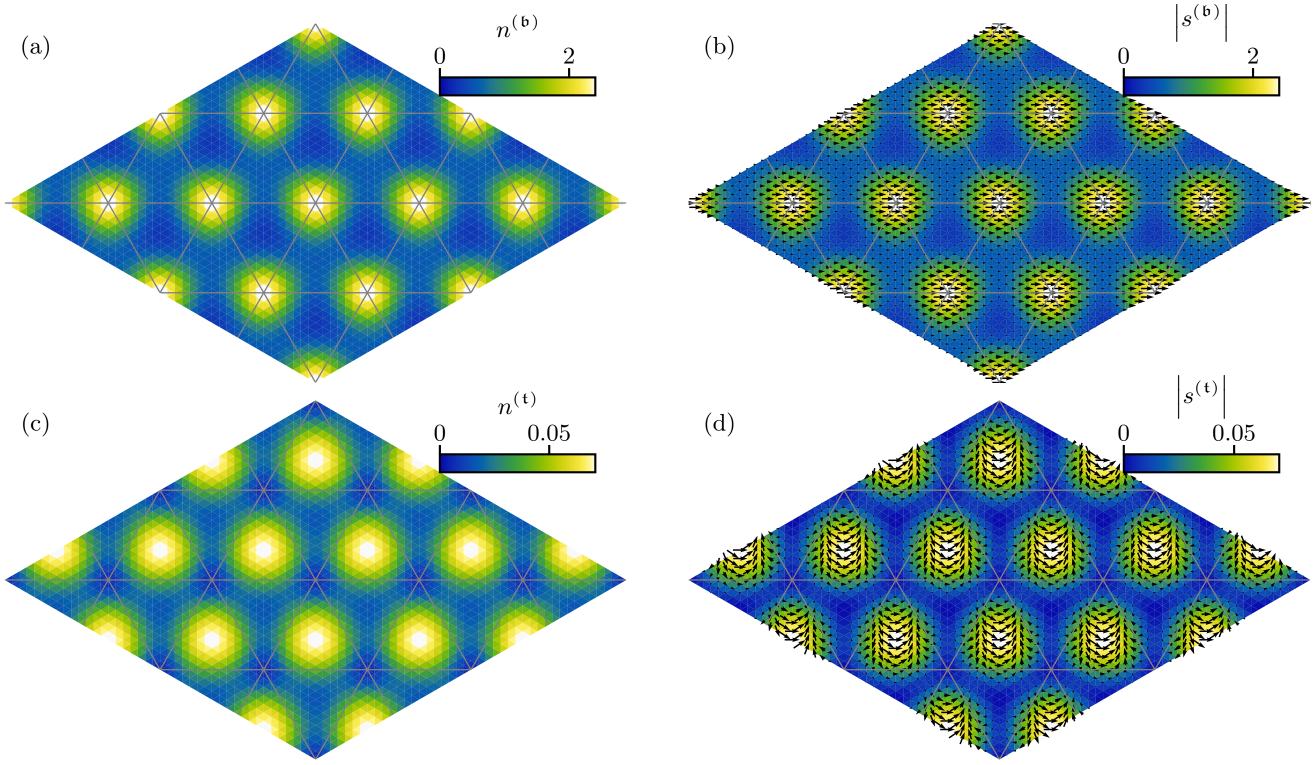


FIG. S4. $\nu = 1$. The charge density waves and spin density waves of $\mathrm{FM}'_x$ at $V_{z\mathfrak{t}} = -20$ meV and $\epsilon = 12$ (although it is not energy favorable compared to competing states at this set of parameters.). The first column shows the hole density $n$ on the bottom (a) and top layer (c); the second column shows the in-plane spin texture with the false color indicating the magnitude on the bottom (b) and top layer (d), respectively($s_z$ vanishes). The gray solid lines connect MM points in the moiré lattice.

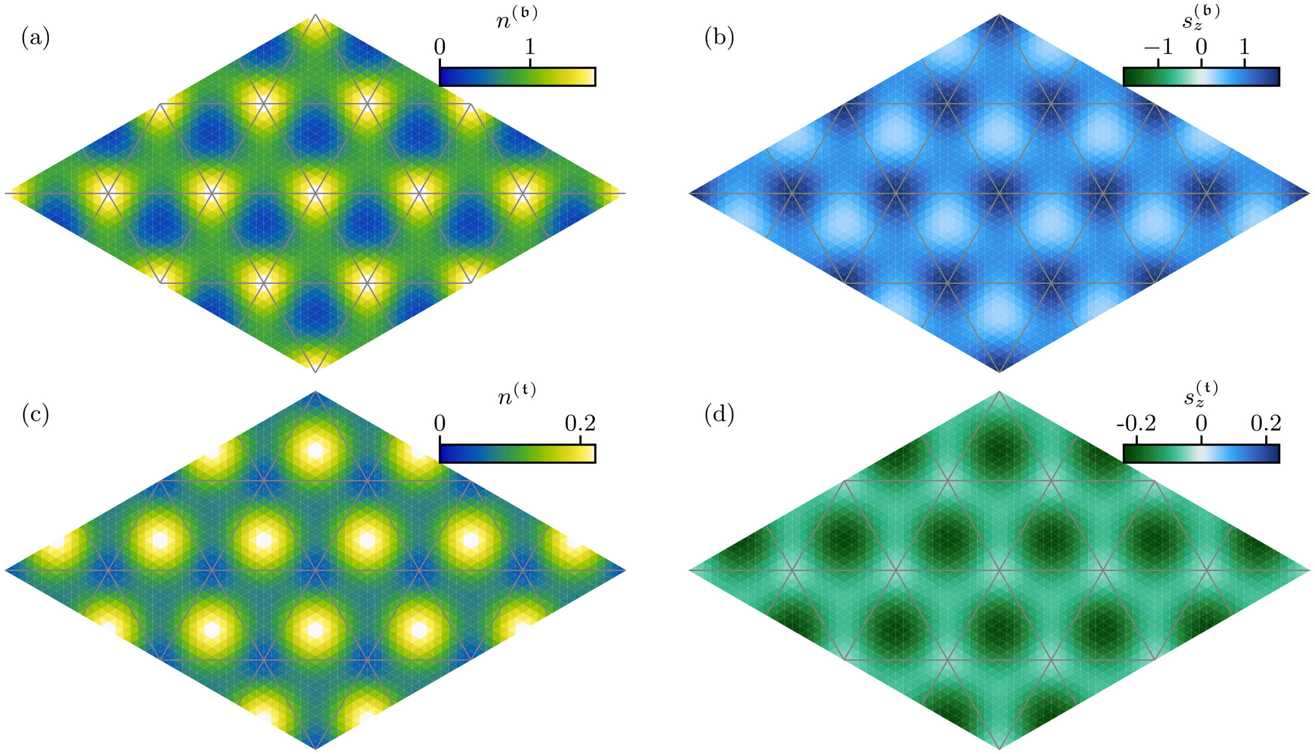


FIG. S5. $\nu = 1$. The charge density waves and spin density waves of valley polarized state at $V_{z\mathfrak{t}} = -20$ meV and $\epsilon = 12$. The first column shows the hole density $n$ on the bottom (a) and top layer (c); the second column shows the out-of-plane spin component $s_z$ on the bottom (b) and top layer (d), respectively. The gray solid lines connect MM points in the moiré lattice.

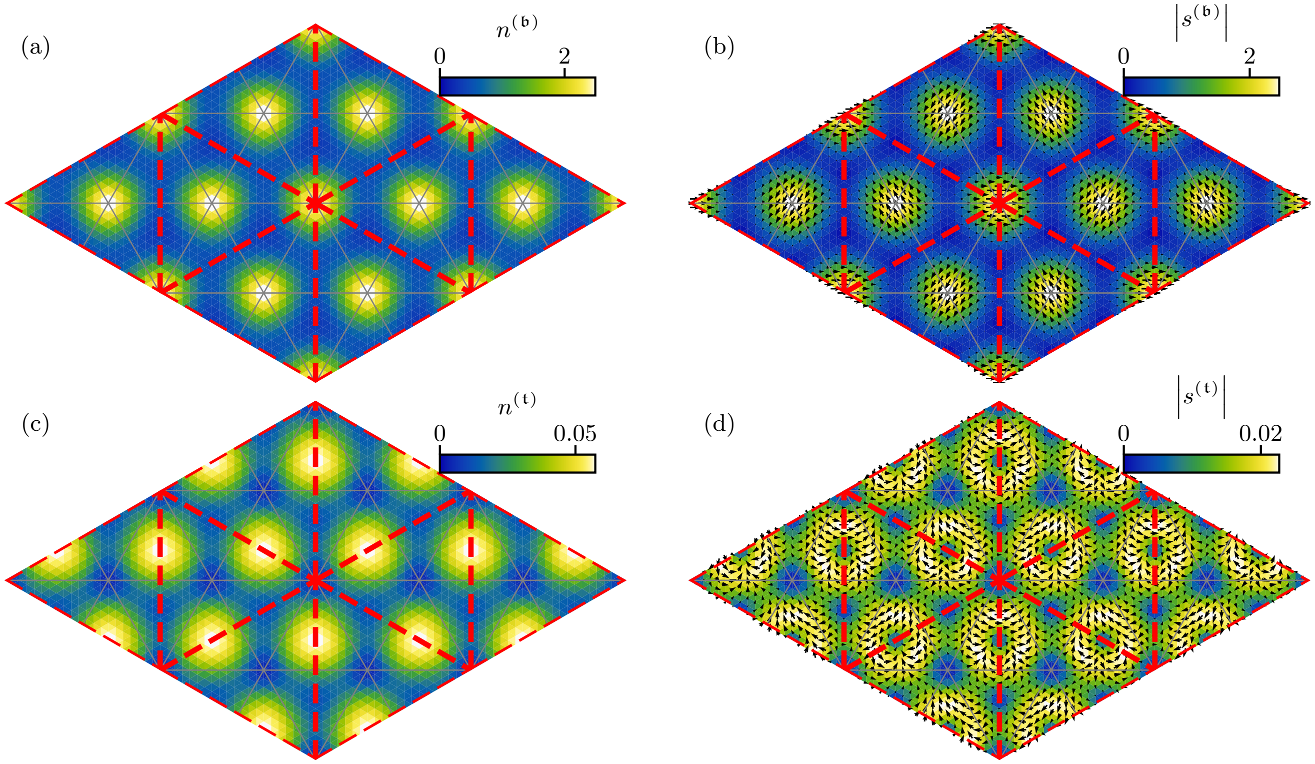


FIG. S6. $\nu = 1$. The charge density waves and spin density waves of the SDW1 at $V_{z\mathfrak{t}} = -10$ meV and $\epsilon = 12$. The first column shows the hole density $n$ on the bottom (a) and top layer (c); the second column shows the in-plane spin texture with the false color indicating the magnitude on the bottom (b) and top layer (d), respectively($s_z$ vanishes). The gray solid lines connect MM points in the moiré lattice, and the red dashed lines show the magnetic unit cell with an enlarged period of $\sqrt{3}a_M$.

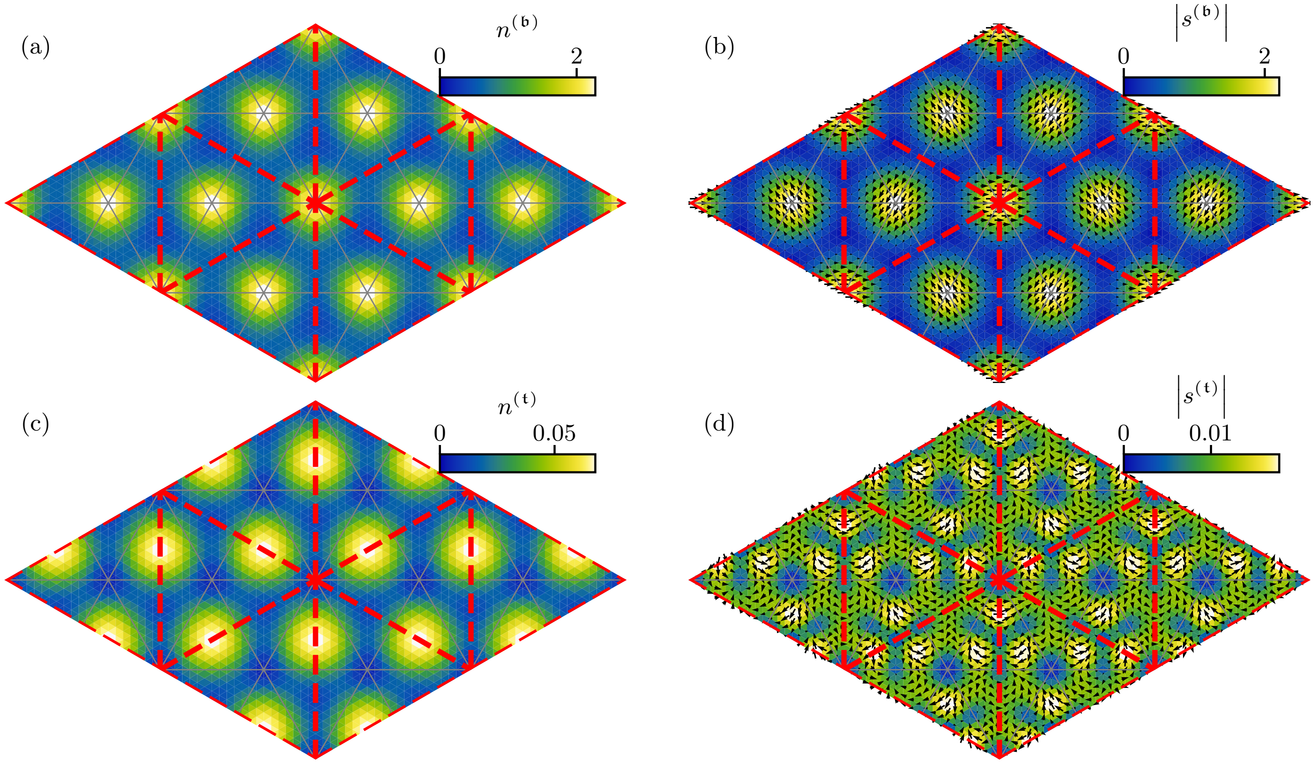


FIG. S7. $\nu = 1$. The charge density waves and spin density waves of the SDW2 at $V_{z\mathfrak{t}} = -20$ meV and $\epsilon = 17$. The first column shows the hole density $n$ on the bottom (a) and top layer (c); the second column shows the in-plane spin texture with the false color indicating the magnitude on the bottom (b) and top layer (d), respectively($s_z$ vanishes). The gray solid lines connect MM points in the moiré lattice, and the red dashed lines show the magnetic unit cell with an enlarged period of $\sqrt{3}a_M$.

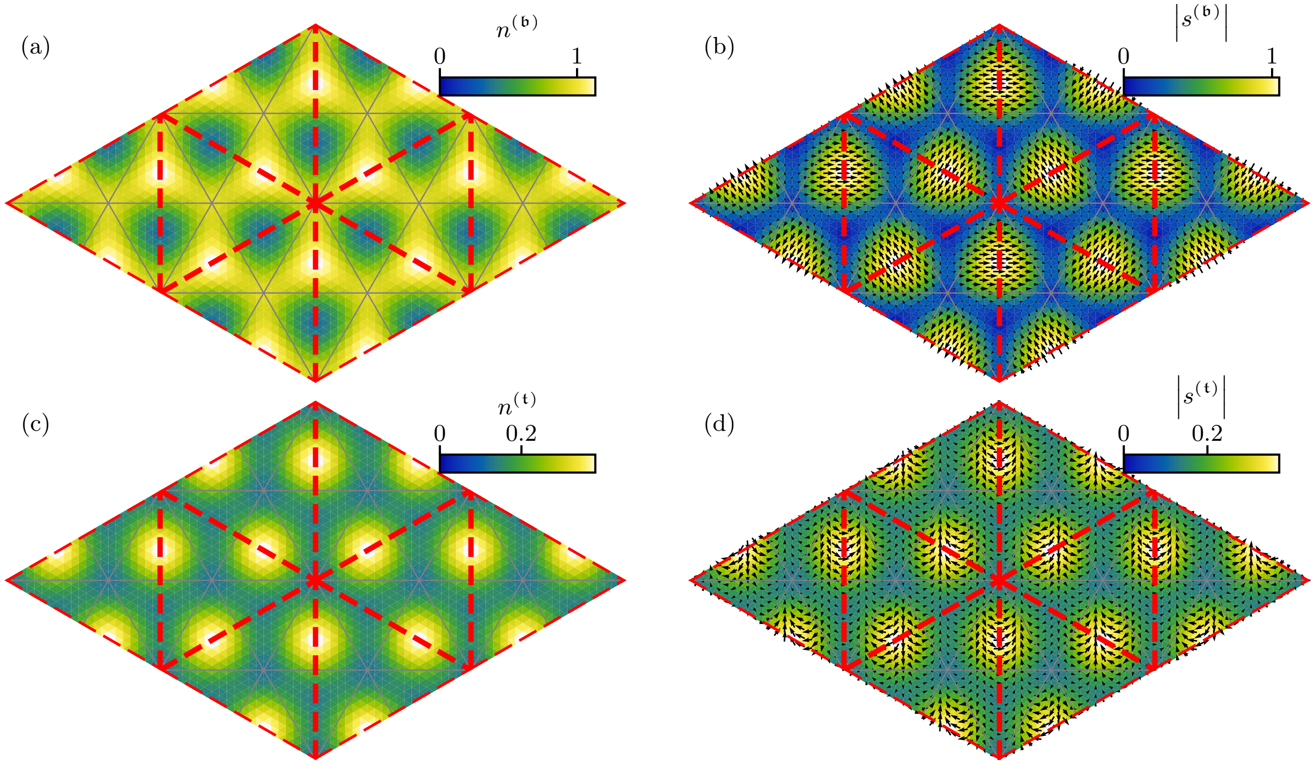


FIG. S8. $\nu = 1$. The charge density waves and spin density waves of the SDW3 at $V_{z\mathfrak{t}} = -10$ meV and $\epsilon = 17$. The first column shows the hole density $n$ on the bottom (a) and top layer (c); the second column shows the in-plane spin texture with the false color indicating the magnitude on the bottom (b) and top layer (d), respectively($s_z$ vanishes). The gray solid lines connect MM points in the moiré lattice, and the red dashed lines show the magnetic unit cell with an enlarged period of $\sqrt{3}a_M$.

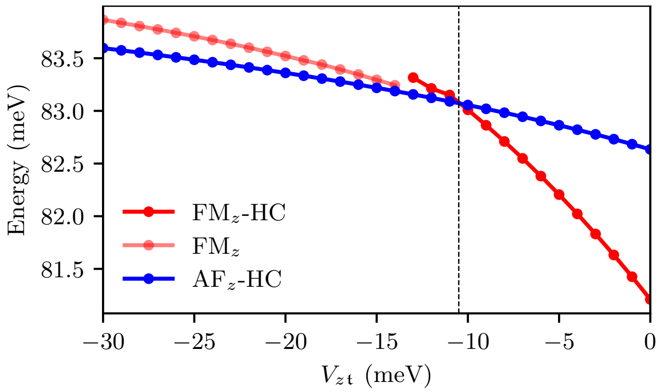


FIG. S9. $\nu = 2/3$. The energies per moiré unit cell of competing states as a function of $V_{z\mathfrak{t}}$ at $\epsilon = 17$. The competing states include AF$_z$-HC (blue), FM$_z$-HC (red) and FM$_z$ (light red).

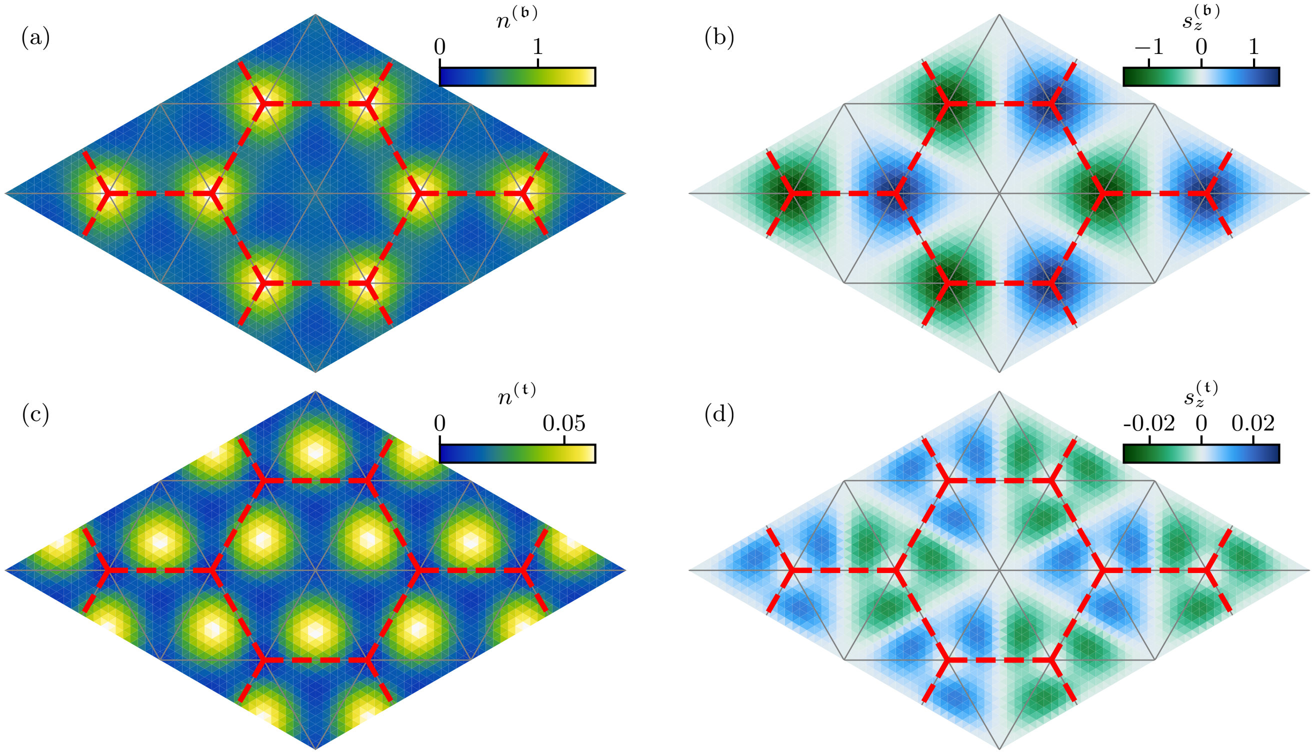


FIG. S10. $\nu = 2/3$. The charge density waves and spin density waves of AF$_z$-HC at $V_{z\mathfrak{t}} = -20$ meV at $\epsilon = 17$. The first column shows the hole density $n$ on the bottom (a) and top layer (c); the second column shows the spin component $s_z$ on the bottom (b) and top layer (d), respectively. The in-plane component of spin is zero. The red dashed lines mark the emergent honeycomb lattice with a period of $\sqrt{3}a_M$.

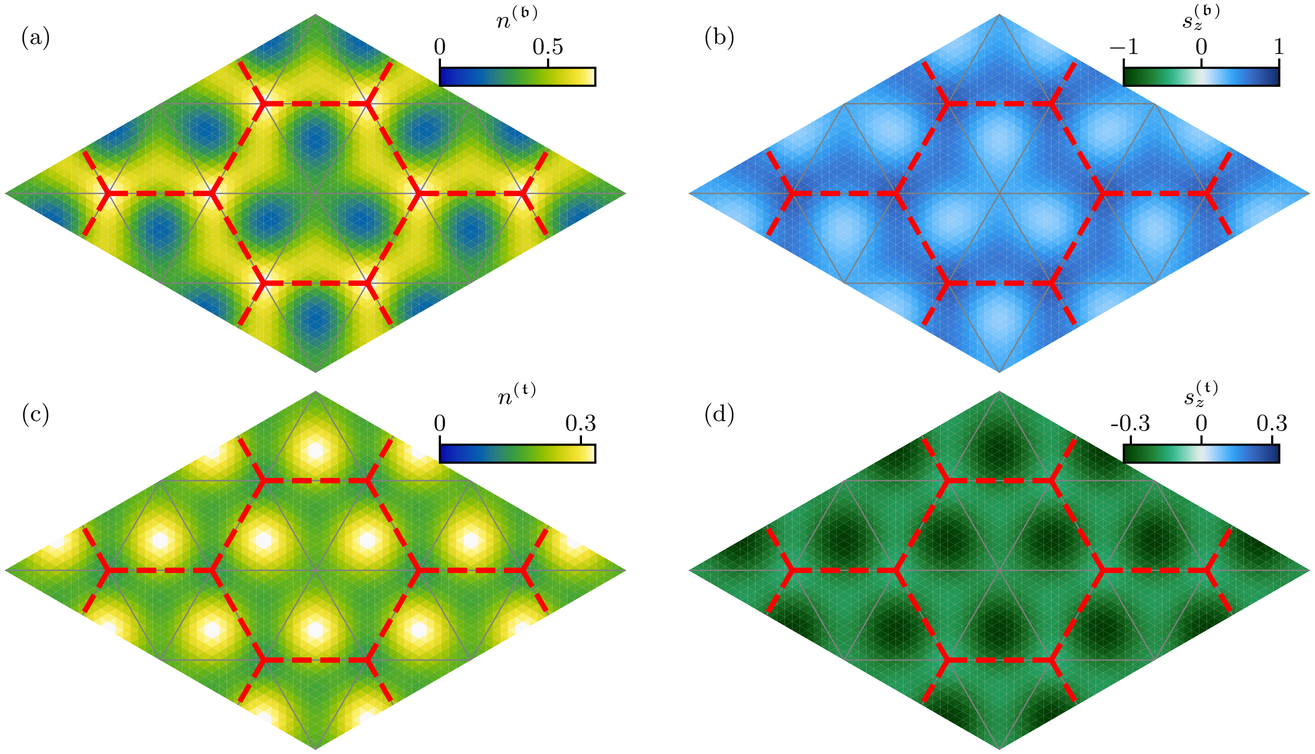


FIG. S11. $\nu = 2/3$. The charge density waves and spin density waves of $\mathrm{FM}_z$-HC at $V_{z\mathfrak{t}} = 0$ meV at $\epsilon = 17$. The first column shows the hole density $n$ on the bottom (a) and top layer (c); the second column shows the spin component $s_z$ on the bottom (b) and top layer (d), respectively. The in-plane component of spin is zero. The red dashed lines mark the emergent honeycomb lattice with a period of $\sqrt{3}a_M$.

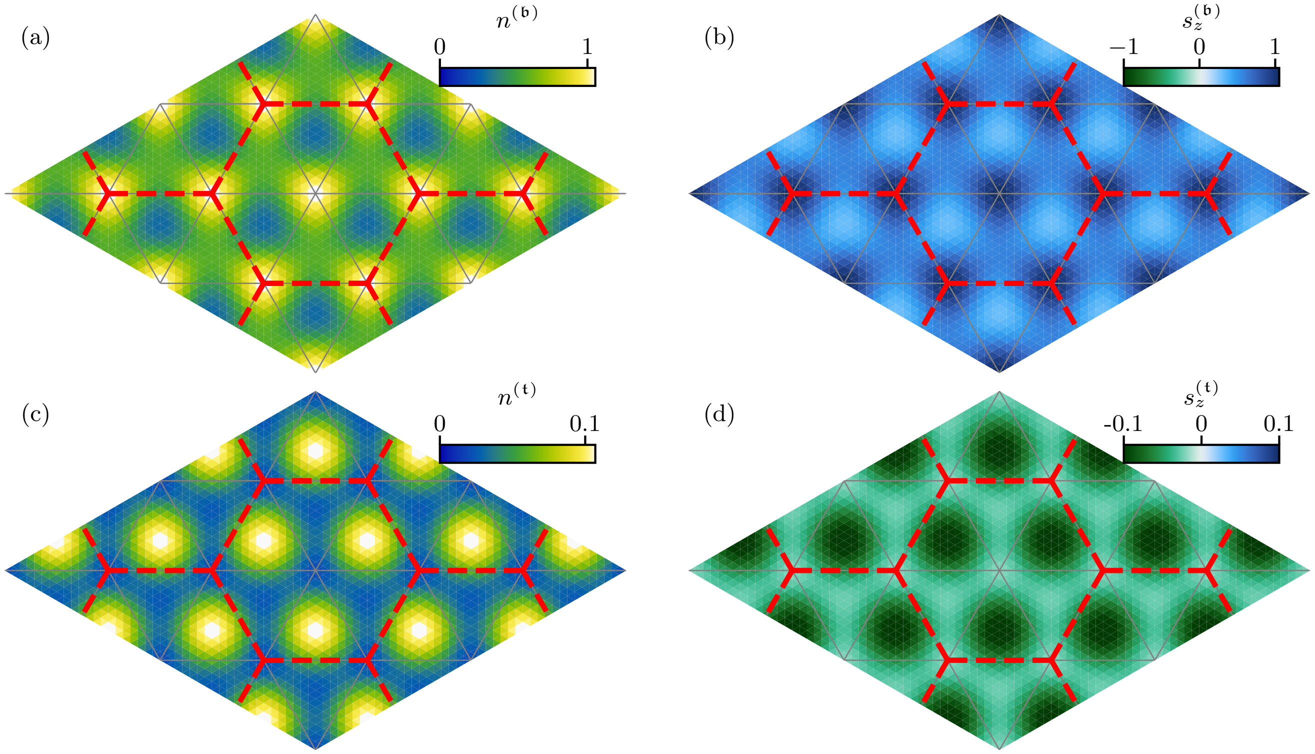


FIG. S12. $\nu = 2/3$. The $\mathrm{FM}_z$ without breaking the moiré lattice translational symmetry at $V_{z\mathfrak{t}} = -16$ meV at $\epsilon = 17$. The first column shows the hole density $n$ on the bottom (a) and top layer (c); the second column shows the spin component $s_z$ on the bottom (b) and top layer (d), respectively. The in-plane component of spin is zero.
